# Supplementary material for: Federated Multi-Task Learning under a Mixture of Distributions
Source: arXiv:2108.10252 source file (2022-11-07)
Supplement: Supplementary file 1 [file broader_impact.tex]

We have proposed new algorithms to learn personalized models. Extensive empirical evaluation shows that our approach learns models not only with higher accuracy, but also higher fairness than state-of-the-art FL algorithms, even for clients not present at training time. 

Federated learning is less efficient than training in a highly-optimized computing cluster. It may in particular increase energy training costs (and thus the carbon footprint), due to a more discontinuous usage of local computing resources and the additional cost of transmitting messages over long distance links. 
Energetic considerations for federated learning have been explored in a few recent papers in different setups \cite{kang19,tran19,carbonFL}.
As our algorithms consume more computation and communication resources per round than other FL algorithms, they may also be more energy-demanding. 
Although we have shown that they can still outperform state-of-the-art methods under the same resource budget, our future work will be oriented to further improve their efficiency. 

Federated learning is intended to protect data privacy, as the data is not collected at a single point. At the same time a federated learning system, as any Internet-scale distributed system, may be more vulnerable to different attacks aiming to jeopardize training or to infer some characteristics of the local dataset by looking at the different messages~\cite{fredrikson2015model,shokri2017membership}.
Encryption \cite{bost2015machine, nikolaenko2013privacy, bonawitz2017practical} and differential privacy \cite{abadi2016deep} techniques may help preventing such attacks. Some features of our algorithms may be beneficial for privacy (e.g., the fact that personalized weights are kept locally and that all users contribute to all shared models).
